# Supplementary material for: Investigating Out-of-Distribution Generalization of GNNs: An Architecture Perspective
Source: arXiv:2402.08228 source file (2024-02-14)
Supplement: Supplementary file 1 [file appendix.tex]

%%%%%%%%%%%%%%%%%%%%%%%%%%%%%%%%

% \begin{table*}[t]
% \setlength{\abovecaptionskip}{0.1cm}
% % \footnotesize
% \centering
% % \setlength{\textfloatsep}{3pt}
% \resizebox{\textwidth}{!}
% {
% % \scalebox{0.59}{
% % \setlength{\tabcolsep}{0.3mm}{
% \begin{tabular}{lllccccccccccccc}
% \toprule[2pt]
% \midrule[1pt]
% \midrule[1pt]
% \multicolumn{3}{c}{\multirow{3}{*}{covariate}} & \multicolumn{4}{c}{GOOD-Cora\textuparrow} & \multicolumn{4}{c}{GOOD-Arxiv\textuparrow} & \multicolumn{2}{c}{GOOD-Twitch\textuparrow} & \multicolumn{2}{c}{GOOD-WebKB\textuparrow} & \multirow{11}{*}{node}\\
% \cmidrule(r){4-7} \cmidrule(r){8-11} \cmidrule(r){12-13} \cmidrule(r){14-15} 

% & & & \multicolumn{2}{c}{word} & \multicolumn{2}{c}{degree} & \multicolumn{2}{c}{time} & \multicolumn{2}{c}{degree} & \multicolumn{2}{c}{language} & \multicolumn{2}{c}{university}  &\\
% \cmidrule(r){4-5} \cmidrule(r){6-7} \cmidrule(r){8-9} \cmidrule(r){10-11} \cmidrule(r){12-13} \cmidrule(r){14-15} 
% & & & \multicolumn{1}{c}{ID\textsubscript{ID}} & \multicolumn{1}{c}{OOD\textsubscript{OOD}} & \multicolumn{1}{c}{ID\textsubscript{ID}} & \multicolumn{1}{c}{OOD\textsubscript{OOD}} & \multicolumn{1}{c}{ID\textsubscript{ID}} & \multicolumn{1}{c}{OOD\textsubscript{OOD}} & \multicolumn{1}{c}{ID\textsubscript{ID}} & \multicolumn{1}{c}{OOD\textsubscript{OOD}} & \multicolumn{1}{c}{ID\textsubscript{ID}} & \multicolumn{1}{c}{OOD\textsubscript{OOD}} & \multicolumn{1}{c}{ID\textsubscript{ID}} & \multicolumn{1}{c}{OOD\textsubscript{OOD}}  &\\
% \cmidrule(r){1-15}

% \multicolumn{3}{l}{ERM} & 70.43 & {64.86} & 72.27 & 56.30 & {72.69} & 71.08 & 77.47 & 58.91 & 70.66 & 48.95 & 38.25 & 14.29 &\\
% \multicolumn{3}{l}{IRM} & 70.27 & 64.77 & {72.64} & 56.28 & 72.66 & 71.04 & 77.50 & 58.98 & 69.75 & 47.21 & 39.34 & 13.49 &\\
% \multicolumn{3}{l}{VREx} & 70.47 & 64.80 & 72.25 & 56.30 & 72.66 & 71.12 & 77.49 & 58.99 & 70.66 & 48.99 & 39.34 & 14.29 &\\
% \multicolumn{3}{l}{GroupDRO} & 70.41 & 64.72 & 72.18 & 56.29 & 72.68 & {71.15} & 77.46 & \textbf{59.08} & 70.84 & 47.20 & 39.89 & 17.20 &\\
% \multicolumn{3}{l}{DANN} & {70.66} & 64.77 & 72.47 & 56.10 & \textbf{72.74} & 71.05 & {77.51} & {59.00} & 70.67 & 48.98 & 39.89 & 15.08 &\\
% \multicolumn{3}{l}{Deep Coral} & 70.47 & 64.72 & 72.16 & {56.35} & 72.66 & 71.07 & 77.48 & 58.97 & 70.67 & 49.64 & 38.25 & 13.76 &\\
% \cmidrule(r){1-15}
% \multicolumn{3}{l}{Mixup} & \textbf{71.54} & \textbf{65.23} & \textbf{74.57} & \textbf{58.20} & 72.49 & \textbf{71.34} & \textbf{77.61} & 57.60 & 71.30 & \textbf{52.27} & \textbf{54.65} & 17.46 &\\
% \multicolumn{3}{l}{EERM} & 68.79 & 61.98 & 73.32 & 56.88 & OOM & OOM & OOM & OOM & \textbf{73.87} & 51.34 & 46.99 & \textbf{24.61} &\\
% \multicolumn{3}{l}{SRGNN} & 70.27 & 64.66 & 71.37 & 54.78 & 72.50 & 70.83 & 75.96 & 57.52 & 70.58 & 47.30 & 39.89 & 13.23 &\\

% \midrule[1.5pt]
% \multicolumn{3}{c}{\multirow{3}{*}{concept}} & \multicolumn{4}{c}{GOOD-Cora\textuparrow} & \multicolumn{4}{c}{GOOD-Arxiv\textuparrow} & \multicolumn{2}{c}{GOOD-Twitch\textuparrow} & \multicolumn{2}{c}{GOOD-WebKB\textuparrow} & \multirow{11}{*}{node}\\
% \cmidrule(r){4-7} \cmidrule(r){8-11} \cmidrule(r){12-13} \cmidrule(r){14-15} 

% & & & \multicolumn{2}{c}{word} & \multicolumn{2}{c}{degree} & \multicolumn{2}{c}{time} & \multicolumn{2}{c}{degree} & \multicolumn{2}{c}{language} & \multicolumn{2}{c}{university}  &\\
% \cmidrule(r){4-5} \cmidrule(r){6-7} \cmidrule(r){8-9} \cmidrule(r){10-11} \cmidrule(r){12-13} \cmidrule(r){14-15} 
% & & & \multicolumn{1}{c}{ID\textsubscript{ID}} & \multicolumn{1}{c}{OOD\textsubscript{OOD}} & \multicolumn{1}{c}{ID\textsubscript{ID}} & \multicolumn{1}{c}{OOD\textsubscript{OOD}} & \multicolumn{1}{c}{ID\textsubscript{ID}} & \multicolumn{1}{c}{OOD\textsubscript{OOD}} & \multicolumn{1}{c}{ID\textsubscript{ID}} & \multicolumn{1}{c}{OOD\textsubscript{OOD}} & \multicolumn{1}{c}{ID\textsubscript{ID}} & \multicolumn{1}{c}{OOD\textsubscript{OOD}} & \multicolumn{1}{c}{ID\textsubscript{ID}} & \multicolumn{1}{c}{OOD\textsubscript{OOD}}  &\\
% \cmidrule(r){1-15}
% \multicolumn{3}{l}{ERM} & 66.05 & {64.60} & {68.71} & 60.54 & 74.76 & 67.32 & \textbf{75.27} & {62.99} & 80.29 & 57.32 & 65.00 & 27.83 &\\
% \multicolumn{3}{l}{IRM} & 66.09 & {64.60} & 68.58 & {61.23} & 74.67 & 67.41 & 75.23 & 62.97 & 77.05 & 59.17 & 65.56 & 27.52 &\\
% \multicolumn{3}{l}{VREx} & 66.00 & 64.57 & 68.45 & 60.58 & {74.80} & 67.37 & 75.19 & \textbf{63.00} & 80.29 & 57.37 & 65.00 & 27.83 &\\
% \multicolumn{3}{l}{GroupDRO} & {66.17} & \textbf{64.62} & 68.37 & 60.65 & 74.73 & \textbf{67.45} & 75.19 & 62.88 & 81.95 & \textbf{60.27} & 65.00 & 28.14 &\\
% \multicolumn{3}{l}{DANN} & 66.16 & 64.51 & 68.08 & 60.78 & 74.73 & 67.28 & {75.25} & 62.91 & 80.28 & 57.46 & 65.00 & 26.91 &\\
% \multicolumn{3}{l}{Deep Coral} & 66.13 & 64.58 & 68.38 & 60.58 & 74.77 & {67.42} & 75.16 & 62.85 & 80.14 & 56.97 & 65.00 & 28.75 &\\
% \cmidrule(r){1-15}
% \multicolumn{3}{l}{Mixup} & \textbf{69.66} & 64.44 & \textbf{70.32} & \textbf{63.65} & \textbf{74.92} & 64.84 & 72.75 & 61.28 & 78.89 & 55.28 & \textbf{67.22} & \textbf{31.19} &\\
% \multicolumn{3}{l}{EERM} & 65.75 & 63.09 & 66.50 & 58.38 & OOM & OOM & OOM & OOM & \textbf{83.91} & 51.94 & 61.67 & 27.83 &\\
% \multicolumn{3}{l}{SRGNN} & 66.45 & \textbf{64.62} & 68.34 & 61.08 & 74.64 & 67.17 & 74.83 & 62.09  & 80.21 & 56.05 & 61.67 & 27.52 &\\

% \bottomrule[2pt]
% \end{tabular}
% }
% \vspace{0.4cm}
% % }
% \caption{ID\textsubscript{ID} and OOD\textsubscript{OOD} performances of 10 baselines on 11 datasets.
% All numerical results are averages across 3 to 10 random runs. Numbers in \textbf{bold} represent the best results. OOM denotes out of memory. Additional results are in Appendix~\ref{sec:D}. More empirical results and analysis are in Appendix~\ref{sec:C}.
% }
% \label{table:OODalgs}
% % \vspace{-10pt}
% \end{table*}
%%%%%%%%%%%%%%%%%%%%%%%%%%%%%%%%%%%%%%%%%%%%%%%%
% \texttt{natbib} 
